# Supplementary material for: CSGO: Content-Style Composition in Text-to-Image Generation
Source: arXiv:2408.16766 source file (2024-09-04)
Supplement: Supplementary file 2 [file 07_appendix.tex]

\section{Details.} 
\subsection{Preliminaries}
\myparagraph{Stable Diffusion. }
The backbone of the stable diffusion model~\cite{DBLP:conf/cvpr/RombachBLEO22} uses CLIP~\cite{radford2021learning} as a text encoder and the UNet structure~\cite{ronneberger2015u} as a latent denoising network. 
%
We refer to the pre-trained UNet as the base model.
%
In general, the U-Net contains multiple down-sampling blocks, a middle block, and multiple up-sampling blocks~\cite{DBLP:journals/corr/abs-2307-01952}. Studies on the controllability of diffusion models usually inject control features into the base model.

\myparagraph{ControlNet. }
% ControlNet~\cite{zhang2023adding} is a large pre-trained text-to-image diffusion model augmented by task-specific image conditions, such as depth map, canny, sketch. 
%
ControlNet models have been developed for image conditions such as depth map, canny, sketch, which effectively enhance the controllability of text-to-image models.
% 
% Taking Stable Diffusion as an example, it is essentially a U-Net~\cite{ronneberger2015u} with some down-sampling blocks, a middle block, and some skip-connected up-sampling blocks. 
%
ControlNet~\cite{zhang2023adding} takes images as the control condition, trains zero-convolution layers and replicates encoder (down-sampling blocks and middle block) of the base model, and injects the resulting outputs of each block into the up-sampling blocks and middle block correspondingly. 
%
Controlnet output features are directly weighted with base model features.

\myparagraph{IP-Adapter. }
% IP-Adapter~\cite{ye2023ip} is widely used by community as image prompting adapter due to its simplicity and effectiveness..
%
IP-Adapter~\cite{ye2023ip} implements image prompt features injected into the text-to-image model by decoupling the cross 
attention module. 
%
In general, image prompts are first obtained as image embeddings by a pre-trained encoder, and then mapped to the key matrix and Value matrix of the attention. Then, they interact with the Query matrix of the base model's attention layer and weight the outputs with the original outputs.
%
IP-Adapter's simplicity and effectiveness in injecting image conditions has received wide attention from the community. 
% In this paper, we make the above feature injection method as \textit{IPAdapter injection}.

\section{More Results.}
